# Supplementary material for: PopALM: Popularity-Aligned Language Models for Social Media Trendy Response Prediction
Source: arXiv:2402.18950 source file (2024-02-29)
Supplement: Supplementary file 1 [file appendix.tex]

\section{Appendix}

\subsection{Original Chinese Content for the Introduction Case}
\label{appendix-Chinese}
We show the original Chinese content of the introduction case in Figure \ref{fig:intro-case-ch}.

\subsection{Original Chinese Content for the Case Study}
\label{case-study appendix-Chinese}

\begin{CJK}{UTF8}{gbsn} 
\begin{table*}[!ht] 
    \resizebox{\columnwidth*2}{!}{%
    \begin{tabular}{p{2\columnwidth}}
        \hline        
        {\bf Post}:
         \ \#哈工大通报志愿者拍考研试卷袋\#：其未接触到试卷拟邀上级部门调查。近日，哈尔滨工业大学
         一志愿者对研究生招生考试试卷袋拍照并发到网上，引发关注。经初步调查，该志愿者工作是在自命题空
         信封上粘贴条形码，全程不能接触到试卷。\\
         \hline

         {\bf ChatGPT:} \ 根据通报中的信息，该志愿者的工作只是在自命题空信封上粘贴条形码，没有接触到真正
         的试卷。学校进行了初步调查，并计划邀请上级部门进行进一步调查，这表明他们对此事件的重视程度。\\
         {\bf ChatGLM:} \ 这条微博的通报信息是准确的，志愿者在考试袋上粘贴条形码并拍照，因此可以排除志愿者
        与考试试卷的接触到的可能性。然而邀请进行上级部门的调查，这可能会引起公众的担忧。\\
         {\bf ChatGLM (P-T):} \ 志愿者是志愿者,考生是考生,都别骂了,这样很没意义。\\
         {\bf ChatGLM (PPO):} \ 别拿志愿者说事了。\\
        {\bf ChatGLM (CL-PPO):} 别搞这些有的没的,该处理处理,该处罚处罚,不要搞什么表面工作。  \\
        \hline
    \end{tabular}
    }
    \caption{The original Chinese content of the
case study.}  
\label{table:caseStudyCh}
\vspace{-5mm}
\end{table*}  
\end{CJK}

The original Chinese content of the case study is shown in Table \ref{table:caseStudyCh}.
\input{pictures/intro-case-ch}

\subsection{Reward modeling}
\label{reward model}
\input{pictures/reward_model}
In Figure \ref{fig: reward model}, we present the performance results of Bert, RoBERTa, and GPT-2 serving as the reward model on the reward test set. From the figure, we observe that GPT-2 and Roberta achieved roughly similar effects, which are somewhat superior to Bert. However, their highest ACC is only around 60\%. This indicates the difficulty of the reward model in predicting which response is trendier when the number of likes is influenced by various factors. Therefore, enhancing the reward signal and selecting high-quality training examples are necessary.
